# Supplementary material for: Uni-HOI:A Unified framework for Learning the Joint distribution of Text and Human-Object Interaction
Source: arXiv:2604.27491 source file (2026-09-11)
Supplement: Supplementary file 1 [file supp.tex]

\documentclass[sigconf,review]{acmart}

\usepackage{xcolor}
\usepackage{multirow}
\usepackage{graphicx}
\usepackage{pifont}

% 解决页眉重叠 + 保持双栏格式
% \pagestyle{plain}
% \AtBeginEnvironment{appendix}{\pagestyle{plain}}

\acmConference[Conference acronym 'XX]{Make sure to enter the correct
  conference title from your rights confirmation email}{June 03--05,
  2018}{Woodstock, NY}
  
\begin{document}

\appendix

% 直接使用 \twocolumn 生成单栏标题，然后继续双栏
\twocolumn[%
    {\centering \Huge \bfseries Appendix \par}
    \vspace{4em}
]

% \appendix
% \twocolumn

\section{Ablation Studies Details}
As shown in Table \ref{tab:ablation}, we conducted ablation experiments to investigate the effects of different model sizes and the use (or absence) of second-stage fine-tuning on the final results. We fix the training hyperparameters and select Qwen3 models of different sizes(Qwen3-1B, Qwen3-4B, Qwen3-8B ) as our backbones for training. We observed that as the model size gradually increased, its performance on multiple HOI tasks improved progressively. This indicates that with larger model sizes, the ability to align text, human motion, and object motion is progressively enhanced, and a larger backbone is more capable of learning the correspondences among the three modalities. Furthermore, compared to performing only the first-stage multi-task training, conducting second-stage task-specific fine-tuning further improves the model's performance on individual tasks.

\section{User Study}
We conducted a user study on the text-to-HOI task to compare our method against other baseline approaches. Twenty text captions covering diverse objects and interaction types were selected, and all four methods were tasked with generating samples based on these captions. Using the results produced by the four methods, we invited 15 participants to select, for each caption, the method that performs best in terms of two criteria: (1) Text Following: which method generates results that best match the input text description; and (2) Contact Details: which method produces results with the most realistic and natural contacts. Figure \ref{fig:user_study} presents the results of the user study, in which our method outperforms the three baselines on both criteria. This demonstrates that our method effectively models the joint distribution between text and HOIs, enabling it to generate more realistic and accurate HOIs.

\begin{figure}[htbp]
    \centering
    \includegraphics[width=0.45\textwidth]{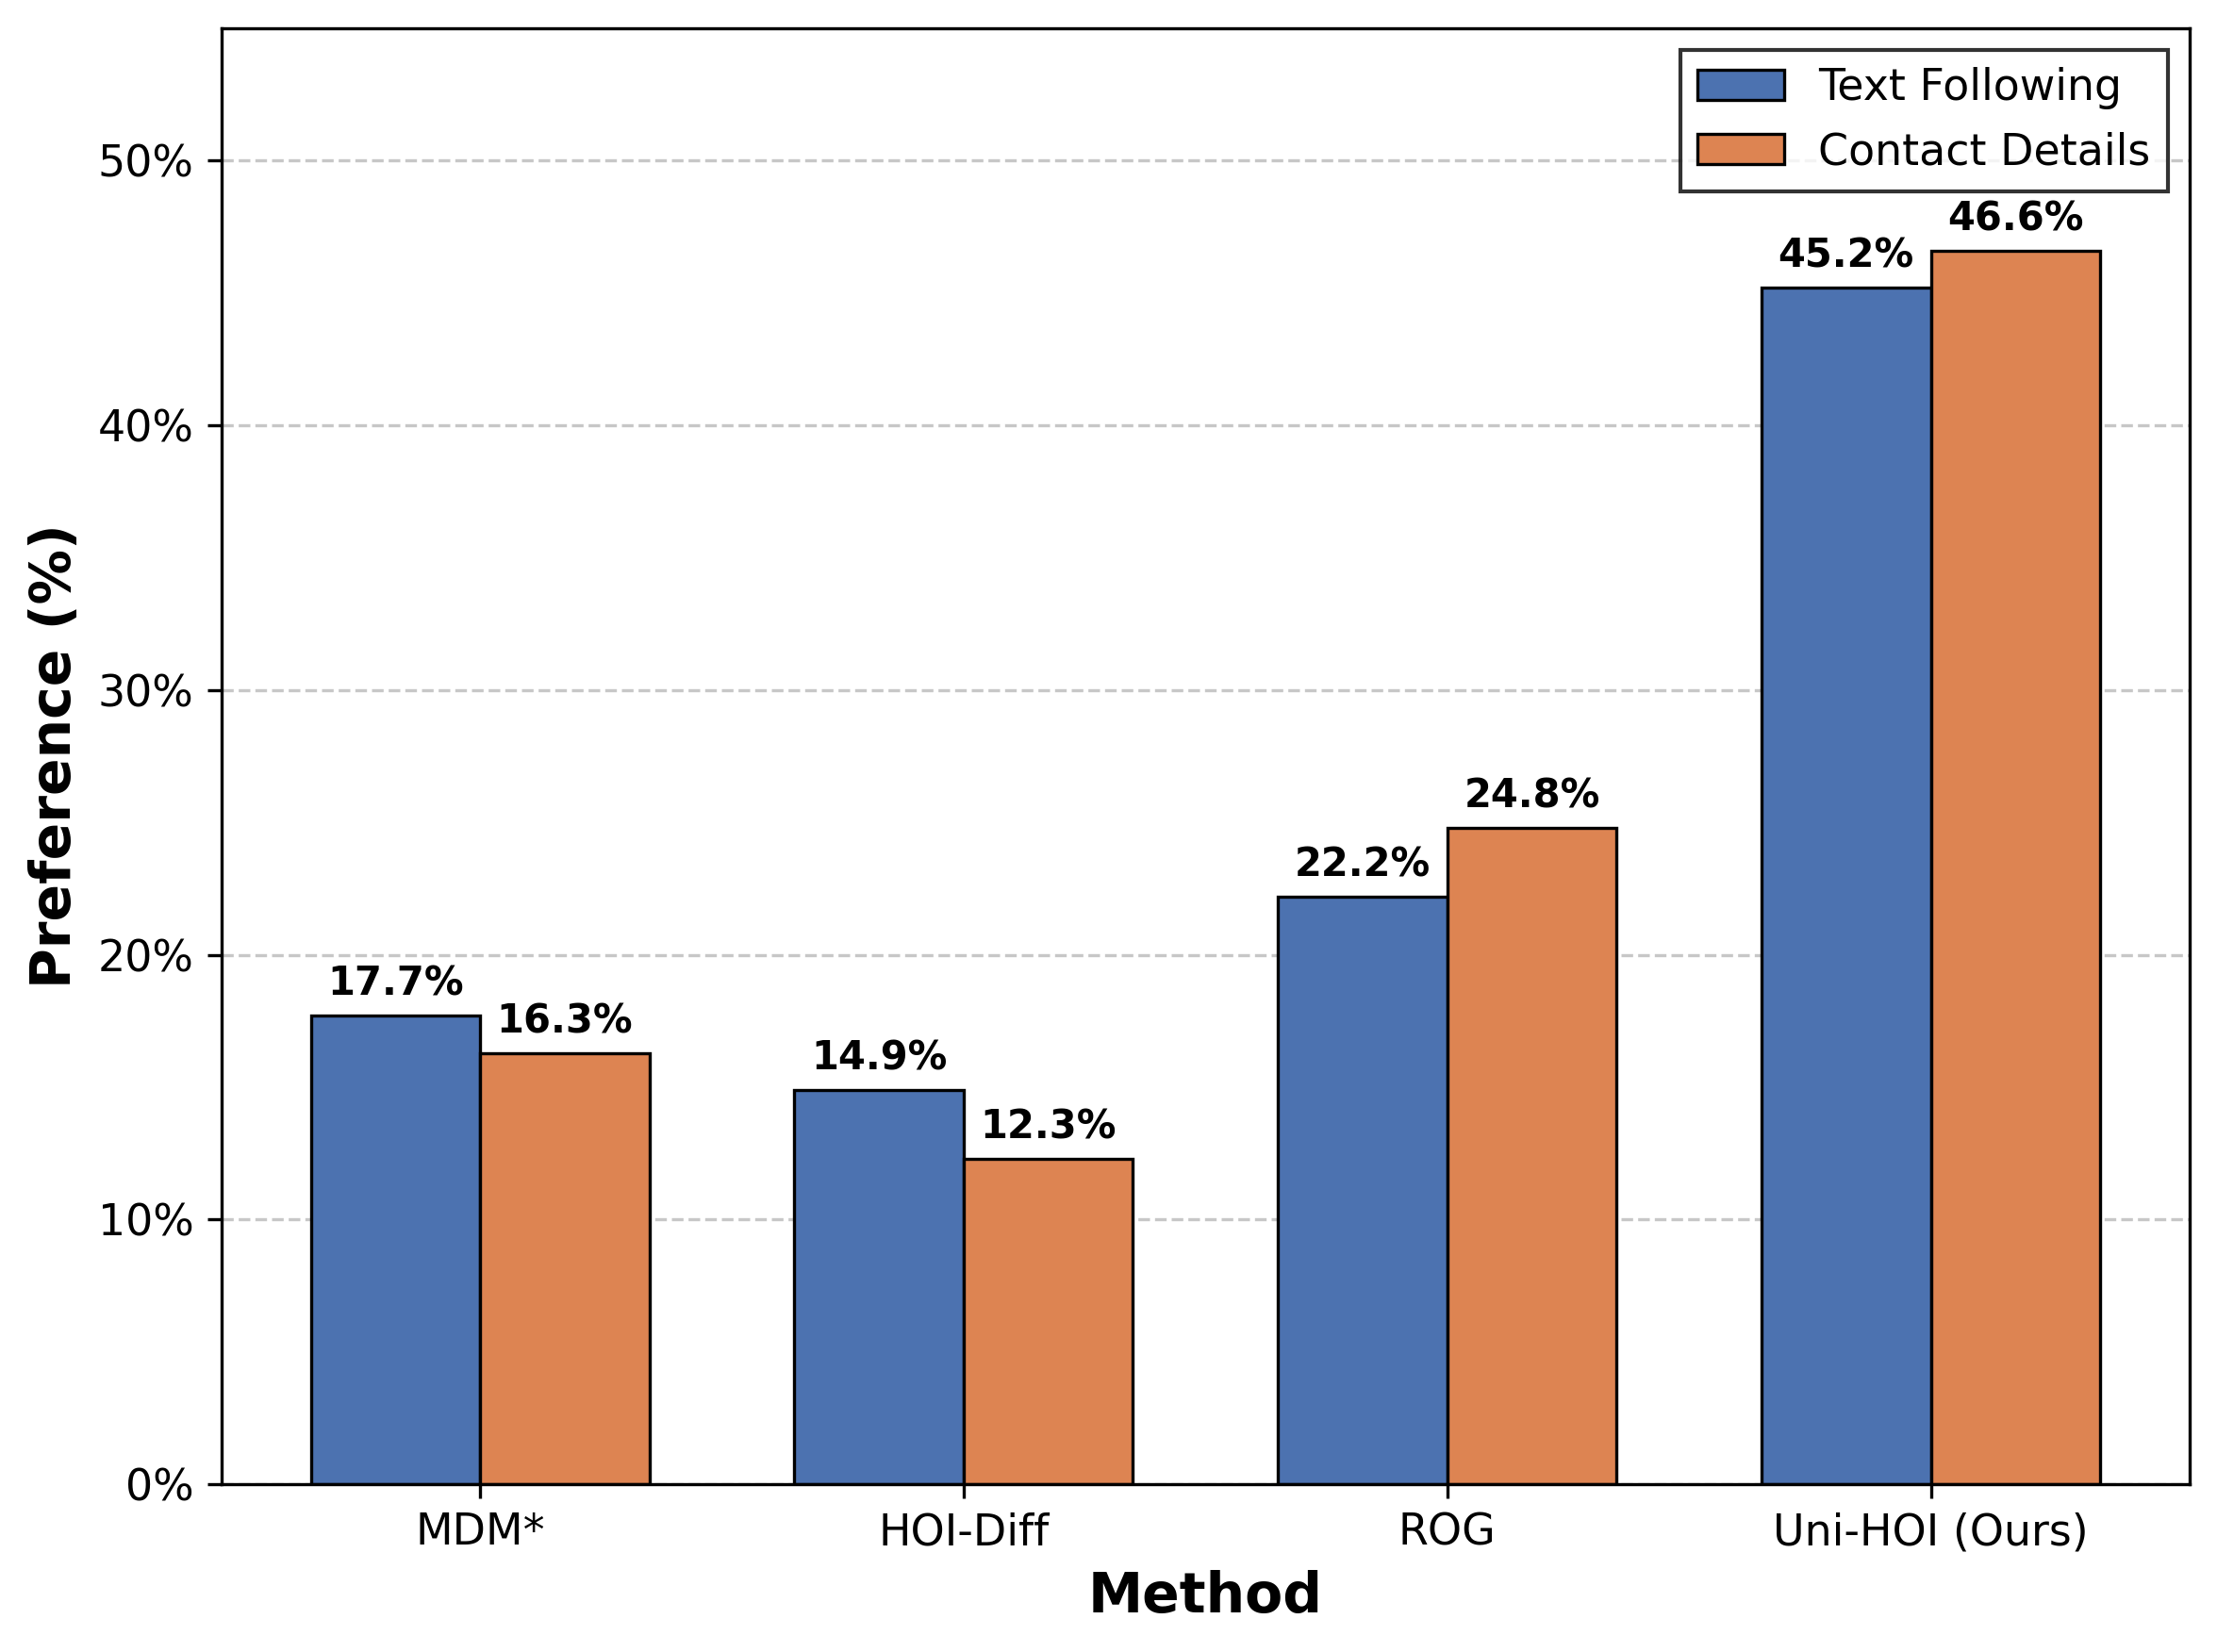}
    \caption{User Study results.}
    \label{fig:user_study}
\end{figure}

\begin{table*}[htbp]
    \centering
    \caption{Ablation studies on the impact of model size and the second-stage task-spcific fine-tuning on multiple HOI-related tasks. $\rightarrow$ means closer to real distribution is better.}
    \setlength{\arrayrulewidth}{0.1em}
    \setlength{\tabcolsep}{5pt}
    \renewcommand{\arraystretch}{1.15}
    
    \begin{tabular}{l@{\hspace{2pt}}c@{\hspace{8pt}}ccc@{\hspace{1em}}ccccc@{\hspace{1em}}ccc}
        \hline
        \multirow{2}{*}{Backbone} & \multirow{2}{*}{Stage-2 Tuning} 
        & \multicolumn{3}{c}{Text-to-HOI} & &\multicolumn{4}{c}{Object-to-Human} & &\multicolumn{2}{c}{Human-to-Object} \\
        % 关键：这三条线会真正断开！
        \cline{3-5} \cline{7-10} \cline{12-13}
        & & FID $\downarrow$ & R Top-3 $\uparrow$ & Div $\rightarrow$ &
        & HandJPE $\downarrow$ & MPJPE $\downarrow$ & $C_{acc}$ $\uparrow$ & $c\%$ $\uparrow$ 
        & & \(E_c\) $\downarrow$ & \(E_{v2v}\) $\downarrow$ \\
        \hline
        GT                & -     & 0.01 &  0.69  & 7.82 &  & -  & -  & -  & -  & & -  & - \\
        \hline
        Qwen3-1B   & \ding{55}  & 6.34  & 0.35  & 9.12  & &33.17  & 19.23  &  0.65 &  0.52 &  & 0.158 & 0.502 \\
        Qwen3-1B  & \ding{51} & 5.87 & 0.42 & 8.69 & &32.46 & 18.52 & 0.72 & 0.60 & & 0.139 & 0.462 \\
        \hline
        Qwen3-4B     & \ding{55}  & 6.13  & 0.40  & 8.76 & & 32.78  & 18.74  & 0.70  & 0.59  & & 0.146  & 0.436 \\
        
        Qwen3-4B     & \ding{51}  & 5.34  & 0.45  & 8.62  & & 31.69  & 17.72  & 0.78  & 0.63 & & 0.127  & 0.374 \\
        \hline
        Qwen3-8B     & \ding{55}  & 5.72  & 0.42  & 8.64 & & 32.15  & 18.56  & 0.76  & 0.62 & & 0.139  & 0.419 \\
        Qwen3-8B(ours)         & \ding{51} & \textbf{5.13} & \textbf{0.55}& \textbf{8.07} & & \textbf{29.87} 
        & \textbf{16.41} & \textbf{0.84} & \textbf{0.72} & & \textbf{0.092} & \textbf{0.325}  \\
        \hline
    \end{tabular}
    \label{tab:ablation}
\end{table*}

\section{Evaluation Details}

Following~\cite{omomo}, we adopt four metrics to quantitatively assess the quality of human-object contact in the generated motion sequences: precision (\(C_{\text{prec}}\)), recall (\(C_{\text{rec}}\)), accuracy (\(C_{\text{acc}}\)), and contact percentage (\(c\%\)).

\vspace{0.5cm}
\noindent  \textbf{Contact Precision (\(C_{\text{prec}}\)).} Precision measures the proportion of predicted contact frames that are actually in contact according to the ground truth. It is defined as:

\begin{equation}
C_{\text{prec}} = \frac{TP}{TP + FP}
\end{equation}

where:
\(TP\) (True Positive) are the frames where both the predicted and ground truth hand positions are within a contact threshold (e.g., 5 cm) from the object surface.
\(FP\) (False Positive) are the frames where the predicted hand is within the threshold but the ground truth is not.
High precision indicates that the model rarely generates false contact signals.

\vspace{0.5cm}
\noindent \textbf{Contact Recall (\(C_{\text{rec}}\)).} Recall measures the proportion of actual ground truth contact frames that are correctly predicted by the model:

\begin{equation}
C_{\text{rec}} = \frac{TP}{TP + FN}   
\end{equation}

where \(FN\) (False Negative) denotes frames where ground truth contact occurs but the predicted hand is beyond the threshold. High recall indicates that the model captures most of the true contact events.

\vspace{0.5cm}
\noindent \textbf{Contact Accuracy (\(C_{\text{acc}}\)).} Accuracy represents the overall correctness of contact prediction across all frames, considering both positive and negative contact frames:

\begin{equation}
C_{\text{acc}} = \frac{TP + TN}{TP + TN + FP + FN}   
\end{equation}

where \(TN\) (True Negative) refers to frames where both the prediction and ground truth indicate no contact. This metric provides a balanced evaluation of the model's ability to correctly identify both contact and non-contact states.

\vspace{0.5cm}
\noindent \textbf{Contact Percentage (\(c\%\)).} The contact percentage quantifies how frequently the generated hand positions are in contact with the object throughout the entire motion sequence:

\begin{equation}
c\% = \frac{\text{Number of frames with predicted contact}}{T} \times 100\%
\end{equation}
\end{equation}

where \(T\) is the total number of frames in the sequence. A frame is considered to have contact if the minimum Euclidean distance between the hand joint and the object mesh surface is below a predefined threshold (e.g., 5 cm).

\vspace{0.5cm}
\noindent \textbf{Vertex-to-Vertex Error.} The vertex-to-vertex error~
\cite{objpop}, denoted as \(E_{\text{v2v}}\), measures the point-wise discrepancy between the predicted object point cloud and the ground truth object point cloud. This metric is applicable when both the predicted and target object representations share the same number of vertices and a consistent vertex correspondence. Formally, given the predicted object vertices \(\mathbf{T}' \in \mathbb{R}^{N \times 3}\) and the ground truth vertices \(\hat{\mathbf{T}}' \in \mathbb{R}^{N \times 3}\), where \(N\) is the number of vertices, the vertex-to-vertex error is computed as the Frobenius norm of their difference:

\begin{equation}
E_{\text{v2v}} = \|\mathbf{T}' - \hat{\mathbf{T}}'\|_F = \sqrt{\sum_{i=1}^{N} \sum_{j=1}^{3} (T'_{ij} - \hat{T}'_{ij})^2}   
\end{equation}

This metric provides a direct per-vertex alignment assessment and is sensitive to both rotational and translational deviations. A smaller \(E_{\text{v2v}}\) indicates better geometric fidelity of the predicted object pose. When the error is computed only for the object centers, we refer to it as \(E_c\), which isolates the translational component of the error.

\vspace{0.5cm}
\noindent \textbf{Chamfer Distance.} When the predicted object and the ground truth object do not share the same number of vertices or vertex correspondence is unavailable, we employ the bidirectional Chamfer distance~\cite{objpop} as an alternative evaluation metric. The Chamfer distance measures the average closest point distance between two point sets, without requiring explicit point-to-point correspondence. Formally, for the predicted point cloud \(\mathbf{T}'\) and the ground truth point cloud \(\hat{\mathbf{T}}'\), the Chamfer distance \(E_{\text{ch}}\) is defined as:

\begin{equation}
E_{\text{ch}} = \frac{1}{|\mathbf{T}'|} \sum_{x \in \mathbf{T}'} \min_{y \in \hat{\mathbf{T}}'} \|x - y\|_2 + \frac{1}{|\hat{\mathbf{T}}'|} \sum_{y \in \hat{\mathbf{T}}'} \min_{x \in \mathbf{T}'} \|y - x\|_2,   
\end{equation}

where \(|\mathbf{T}'|\) and \(|\hat{\mathbf{T}}'|\) denote the number of points in the predicted and ground truth point clouds, respectively. The first term computes the average distance from each predicted point to its nearest neighbor in the ground truth set, measuring completeness; the second term computes the average distance from each ground truth point to its nearest neighbor in the predicted set, measuring accuracy.

\section{Details for Object Geometry Token}

We design a lightweight point cloud feature extractor for encoding 3D object geometry. Given an input point cloud \(\mathbf{P} \in \mathbb{R}^{N \times 3}\), the network outputs a global feature embedding \(\mathbf{f} \in \mathbb{R}^{1 \times 4096}\).

The architecture comprises three stages. First, per-point features are extracted through three 1D convolutional layers with kernel size 1, progressively increasing the channel dimension from 3 to 64, 128, and 256. Each convolution is followed by GroupNorm (with a single group) and ReLU activation. Second, symmetric pooling is applied along the point dimension: max pooling and average pooling capture complementary statistics, and their outputs (each \( \in \mathbb{R}^{256}\)) are concatenated into a  global feature vector( \( \in \mathbb{R}^{512}\)). Third, a three-layer MLP transforms this vector to the target dimension of 4096, with GroupNorm and ReLU applied after the first two layers.

GroupNorm replaces BatchNorm to ensure stable training with small batch sizes (e.g., batch size 1). The combination of max and average pooling provides permutation invariance while preserving both salient local features and global point distribution statistics. The network contains approximately 24 million parameters, offering a compact yet expressive representation for object geometry in human-object interaction tasks.

\begin{figure*}[htbp]
    \centering
    \includegraphics[width=0.8\textwidth]{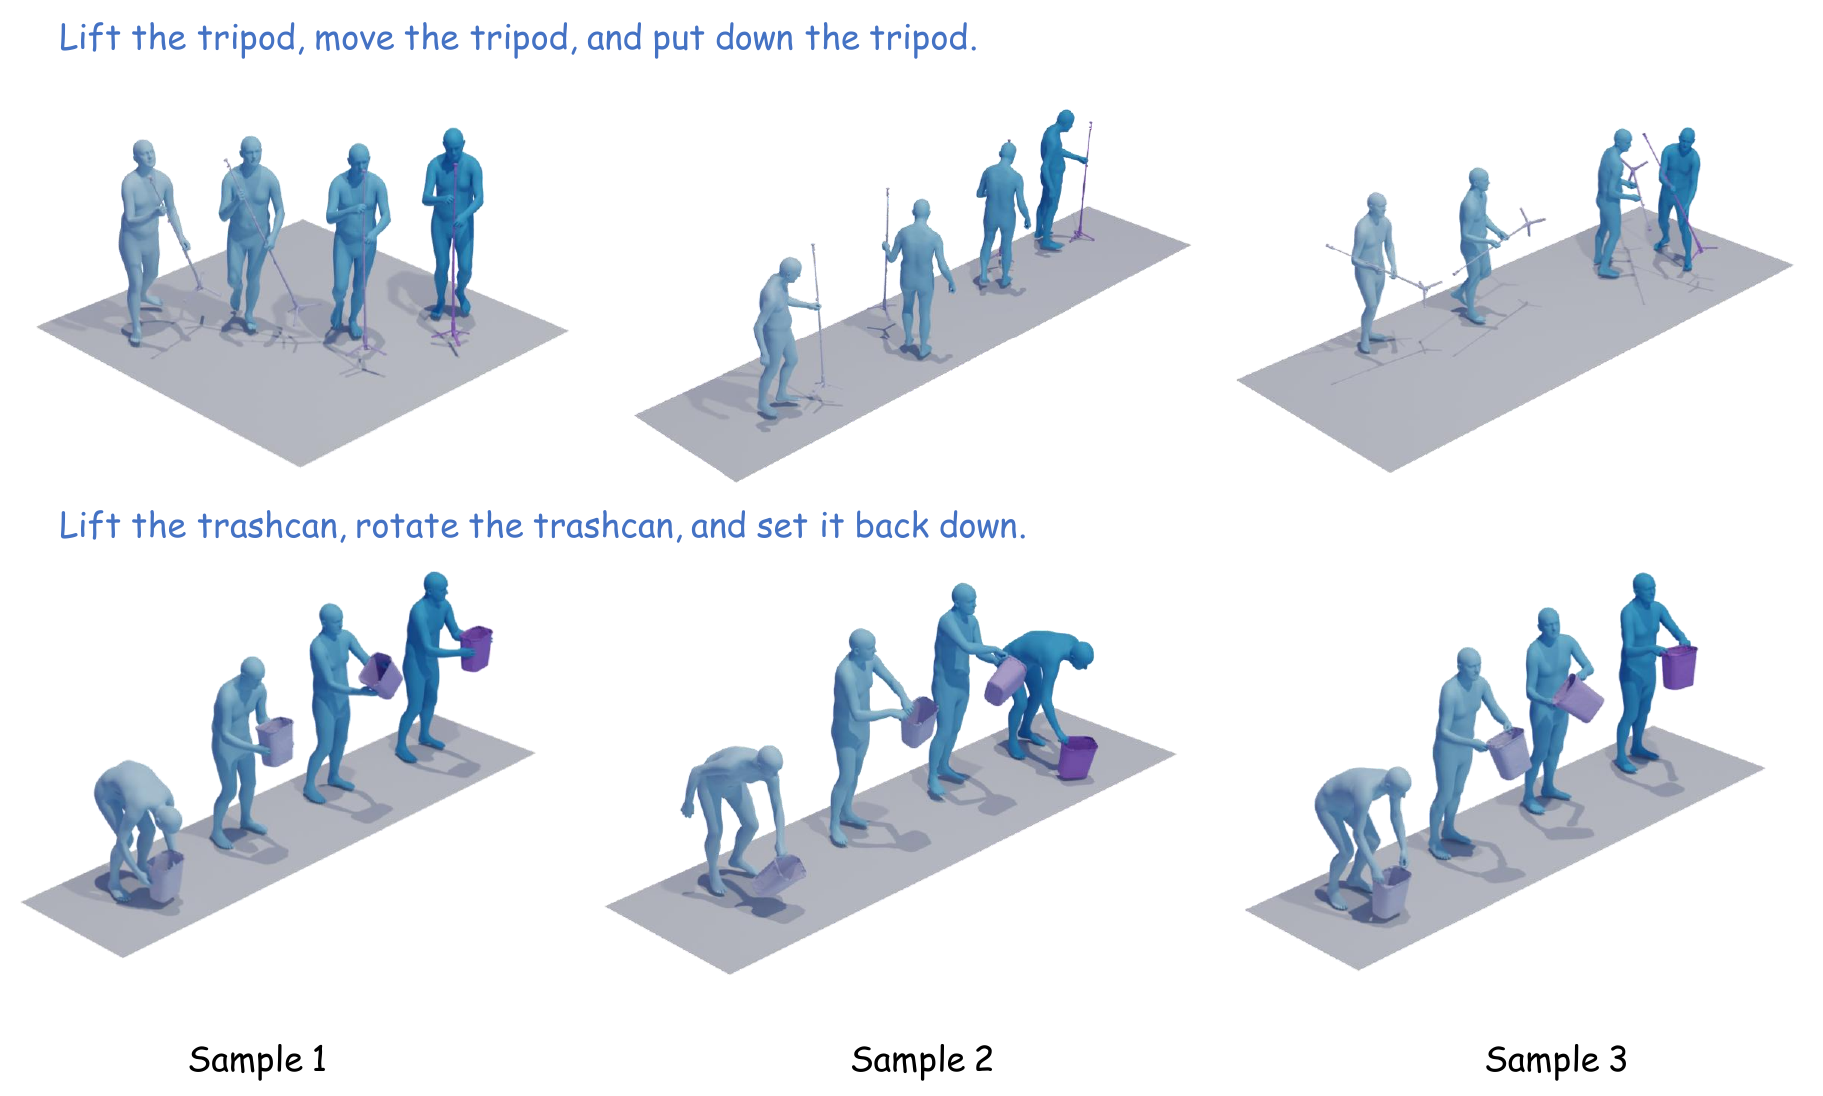}
    \caption{Given a text prompt, our model is capable of generating multiple distinct and naturally plausible HOI results. }
    \label{fig:diversity}
\end{figure*}

\begin{figure*}[htbp]
    \centering
    \includegraphics[width=\textwidth]{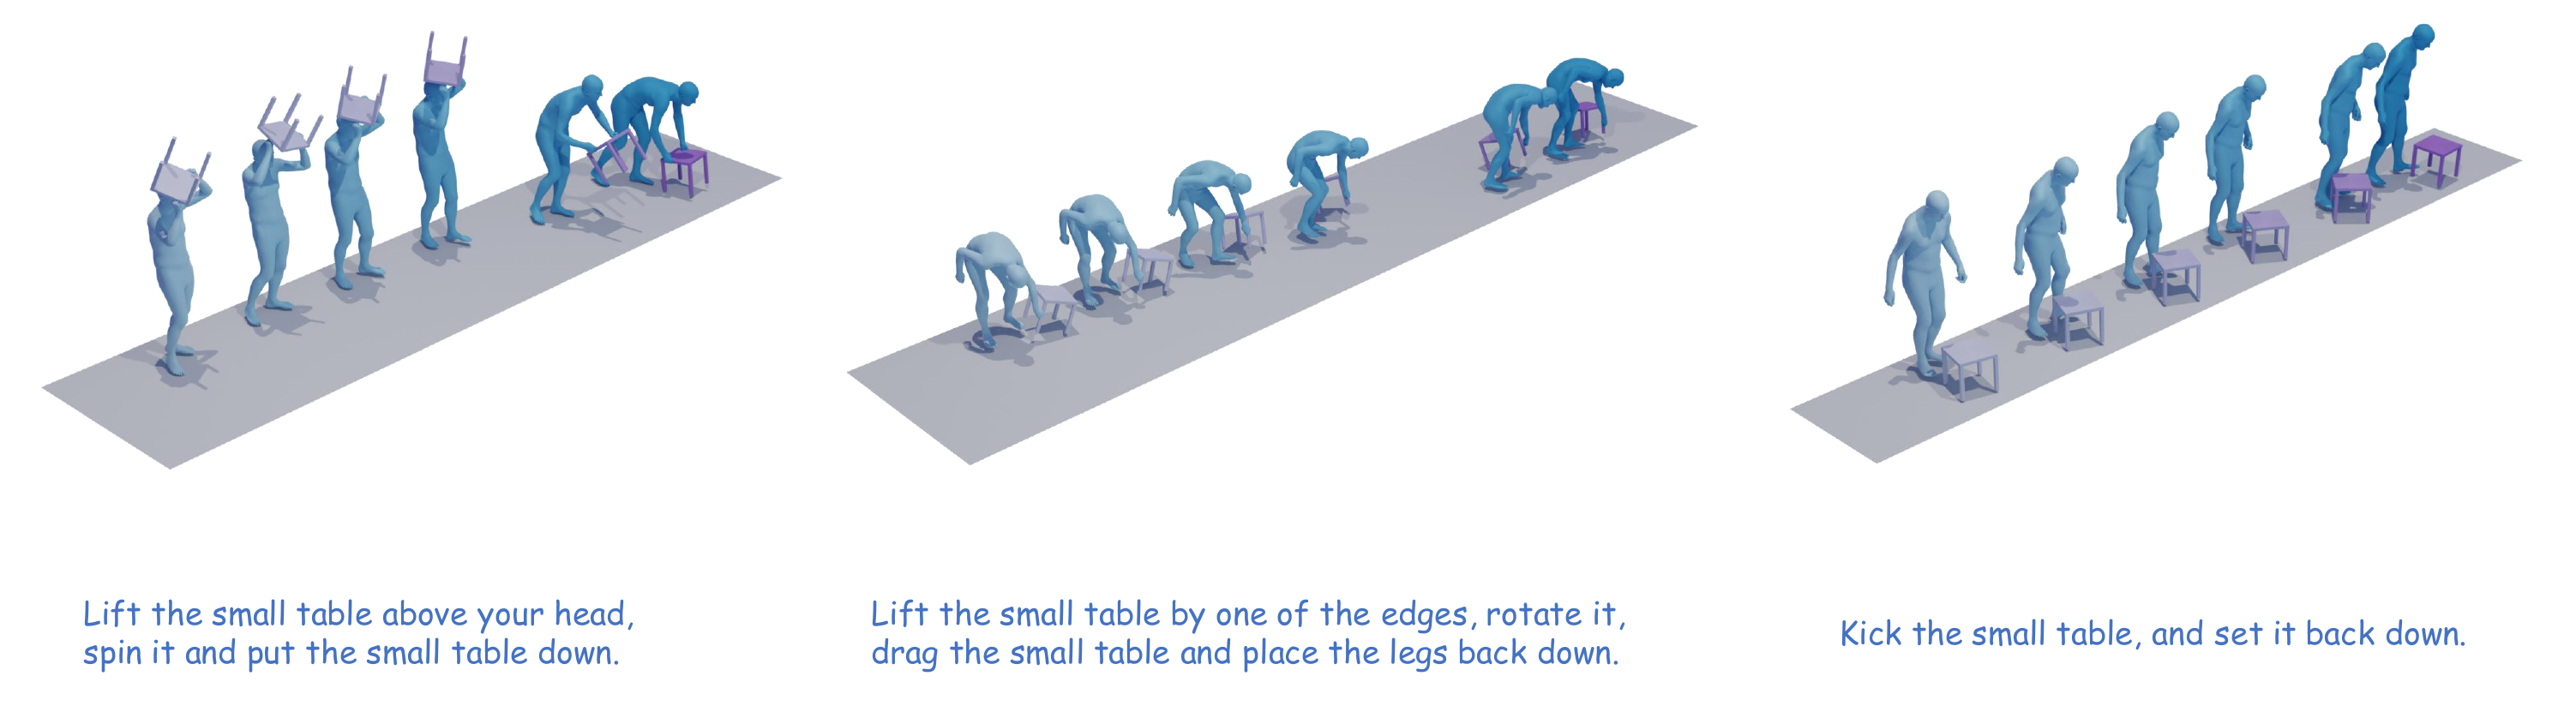}
    \caption{Our model generates diverse, semantically distinct human-object interactions for a single object. }
    \label{fig:diverse_same_object}
\end{figure*}

\begin{figure*}[htbp]
    \centering
    \includegraphics[width=0.85\textwidth]{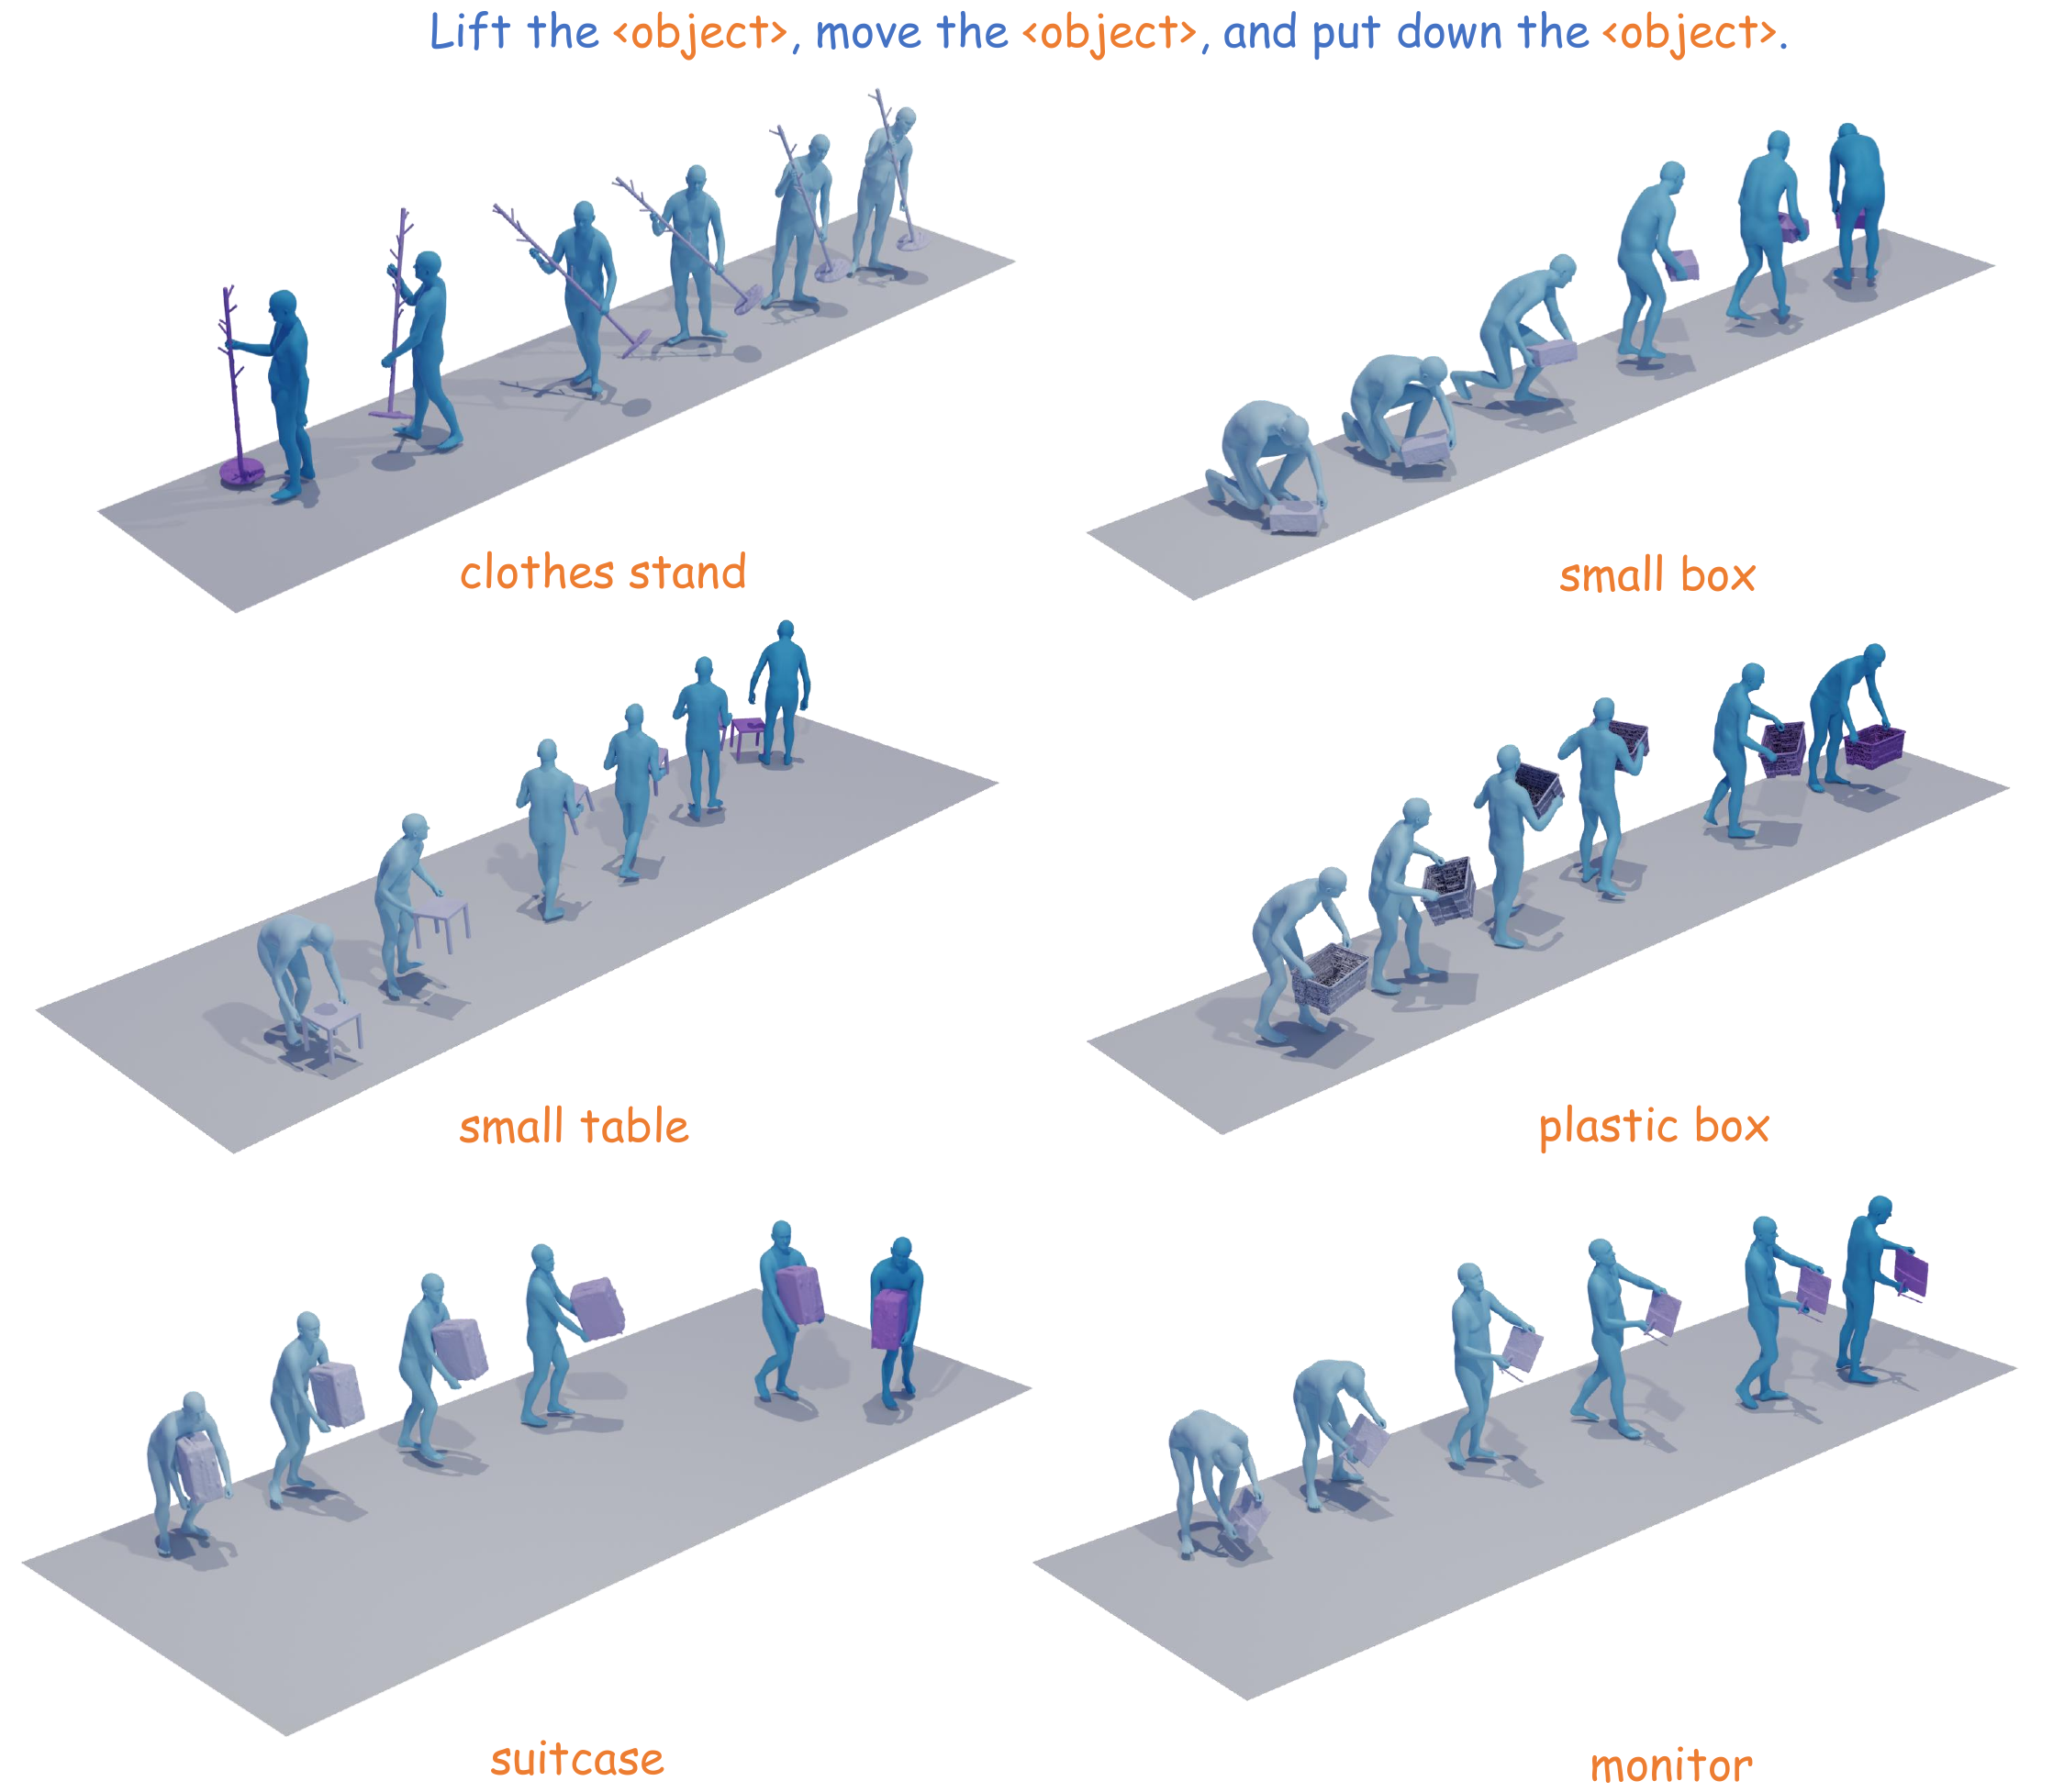}
    \caption{Our model generates semantically accurate and consistent human-object interactions across a diverse set of objects. }
    \label{fig:diverse_object}
\end{figure*}

\begin{figure*}[htbp]
    \centering
    \includegraphics[width=\textwidth]{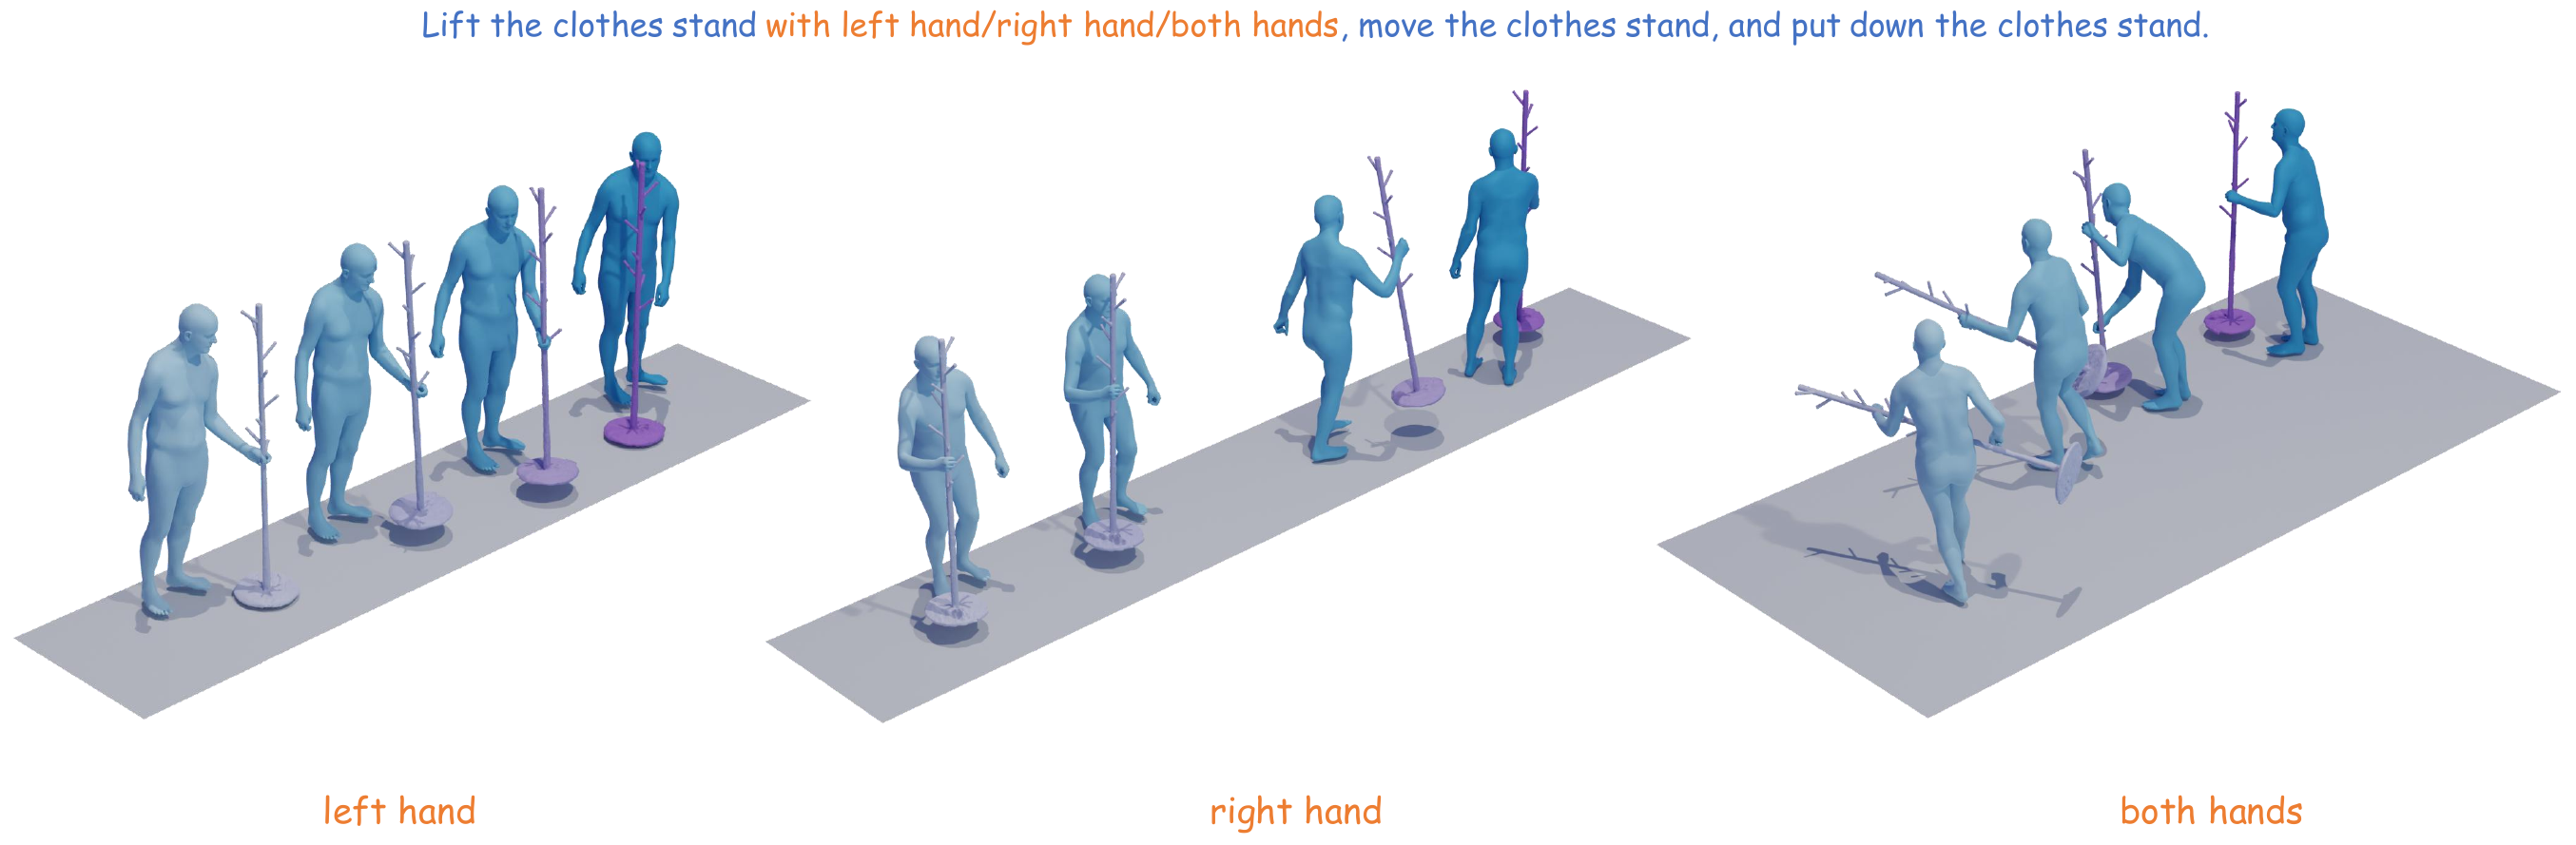}
    \caption{Our model can generate HOI consistent with the description based on the specific interacting body parts specified by the prompt.}
    \label{fig:diverse_interaction}
\end{figure*}

\begin{figure*}[htbp]
    \centering
    \includegraphics[width=\textwidth]{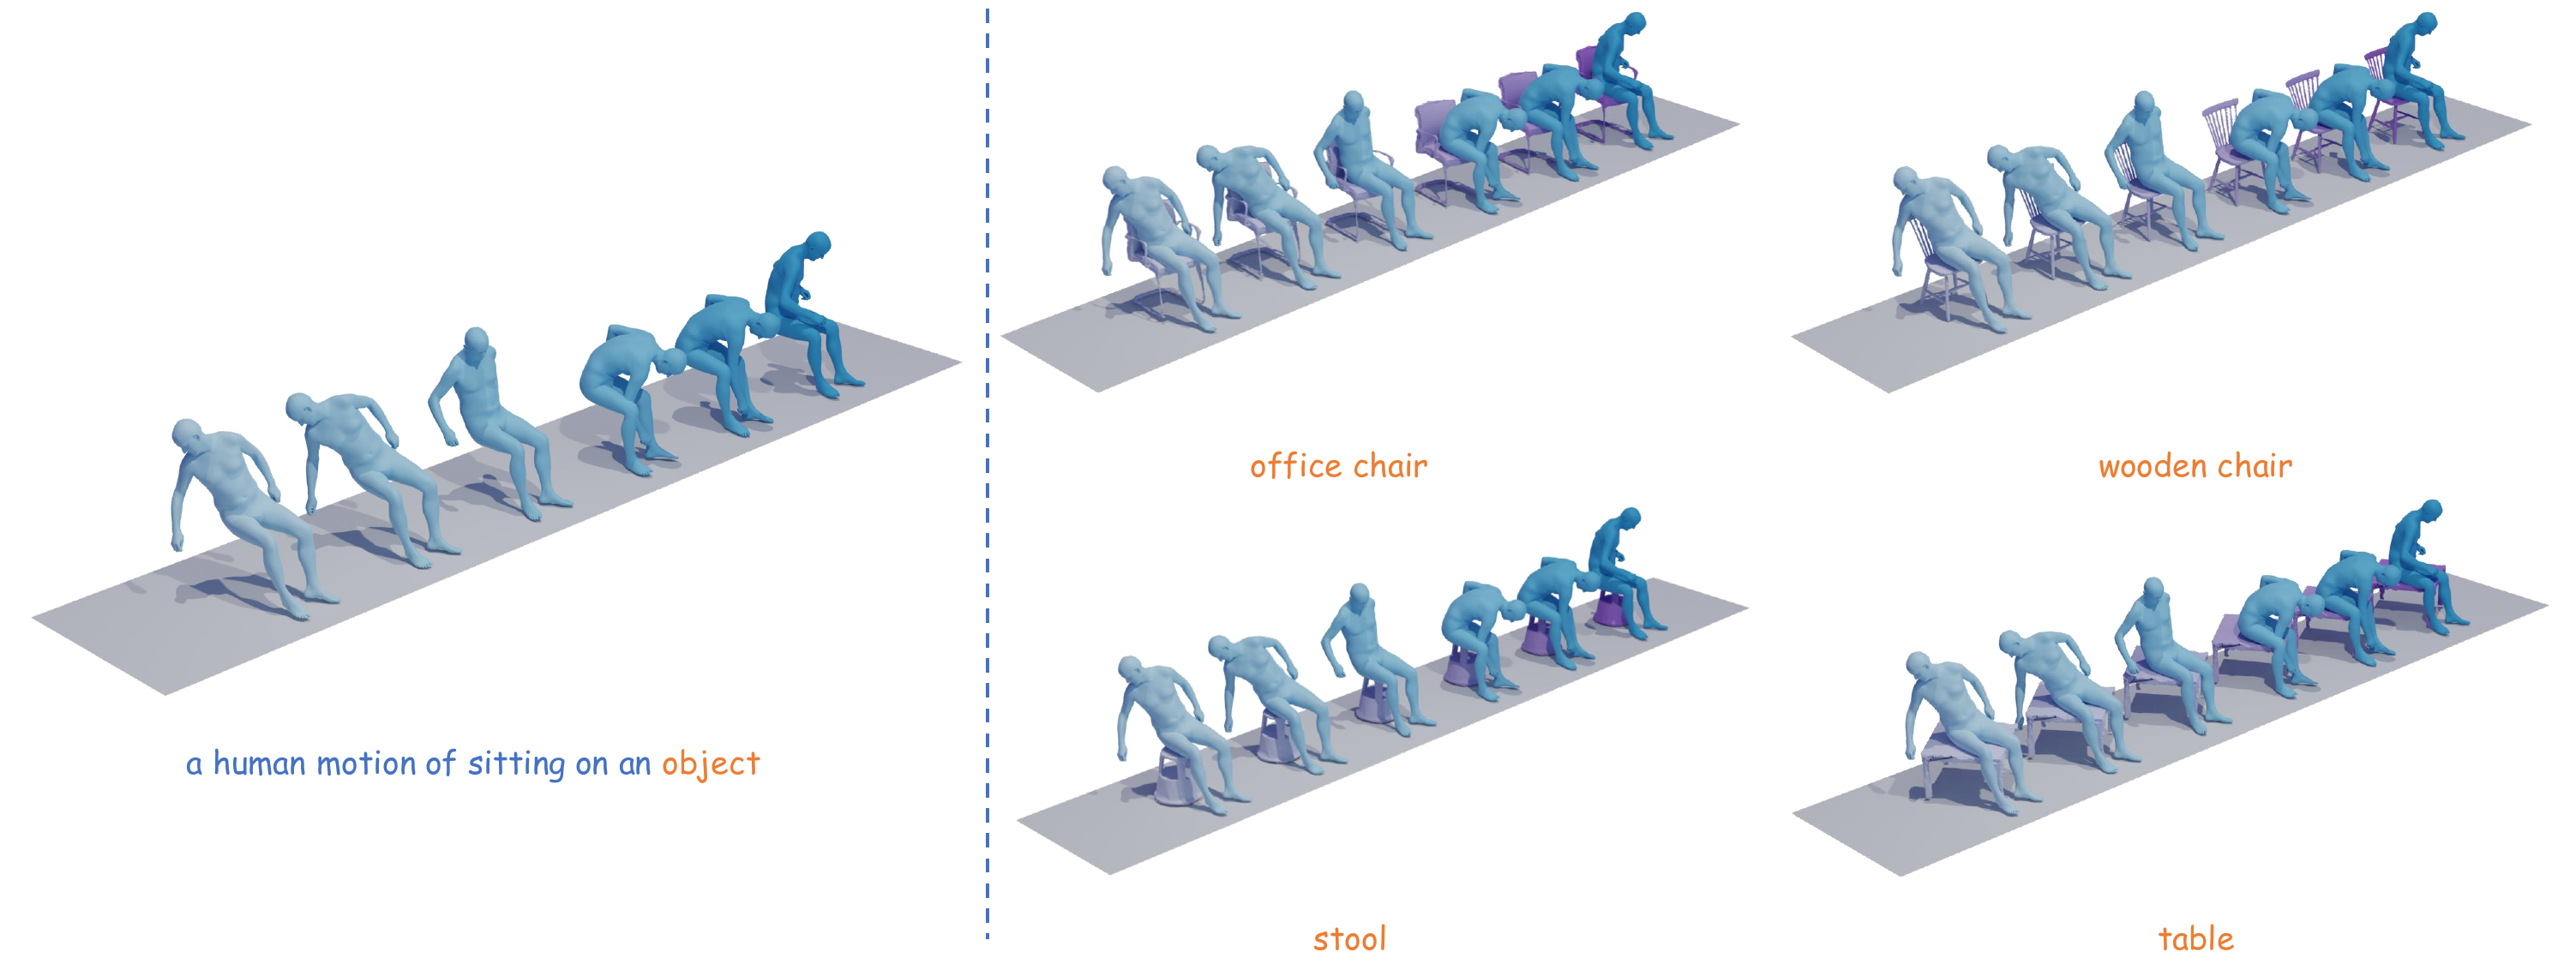}
    \caption{Given a human motion sequence and the meshes of various objects, our model accurately predicts the motion of different objects, thereby synthesizing realistic and plausible HOI.}
    \label{fig:diverse_sit}
\end{figure*}

\section{Additional Qualitative Results}

\vspace{0.5cm}

\noindent \textbf{Diverse results with the Same Prompt.} We evaluate the diversity generation capability of our model under identical conditions. As illustrated in Figure \ref{fig:diversity}, for the same text input, our model is able to generate diverse and realistic HOI sequences, demonstrating the strong potential of our framework in producing diverse and requirement-satisfying results for users.

\vspace{0.5cm}
\noindent \textbf{Diverse Interactions with the Same Object.}
We evaluate the ability of our model to generate diverse interactions for the same object. Using a small table as an example, Figure \ref{fig:diverse_same_object} illustrates a range of motions, including "lift the object above the head," "Lift the object by one of the edges," and "kick the object." These results demonstrate the flexibility of our approach in producing semantically distinct and contextually appropriate interactions with a single object.

\vspace{0.5cm}
\noindent \textbf{Consistent Interaction on Different Objects.} We evaluate the ability of our method to generate consistent motion sequences across diverse scenarios, specifically focusing on the task chain of "lift the object, move the object, and put down the object" as applied to various objects. Figure \ref{fig:diverse_object} presents the visualized results for 6 distinct objects: a clothes stand, a small box, a small table, a plastic box, a suitcase and a monitor. These examples collectively demonstrate that Uni-HOI is capable of producing semantically accurate and temporally consistent interactions across a broad range of object types.

\vspace{0.5cm}
\noindent \textbf{Prompt-aligned Interaction on Specified Body Parts.} 
We further validate the capability of our model to generate fine-grained interactions within the text-to-HOI task. By specifying precise interacting body parts in the text prompt—for instance, utilizing the left hand, right hand, or both hands to engage with the object—we demonstrate that our model produces HOI sequences with high fidelity to the described interaction details, as illustrated in Figure \ref{fig:diverse_interaction}. These results underscore the superior performance of our model in generating fine-grained HOI.

\vspace{0.5cm}
\noindent \textbf{Object Motion Prediction for Novel Object.} We explore the generalization capability of our model to diverse object geometries in the object motion prediction task. Given a human motion sequence depicting a person sitting on an office chair, we replace the input object with a wooden chair, a stool, and a table for evaluation. As illustrated in Figure 5, our model successfully predicts the motion of objects with varying geometric configurations, synthesizing realistic HOI sequences in each case.

\bibliographystyle{ACM-Reference-Format}
\bibliography{sample-base}

\end{document}
